# Supplementary material for: Multi-Granularity Video Object Segmentation
Source: arXiv:2412.01471 source file (2024-12-03)

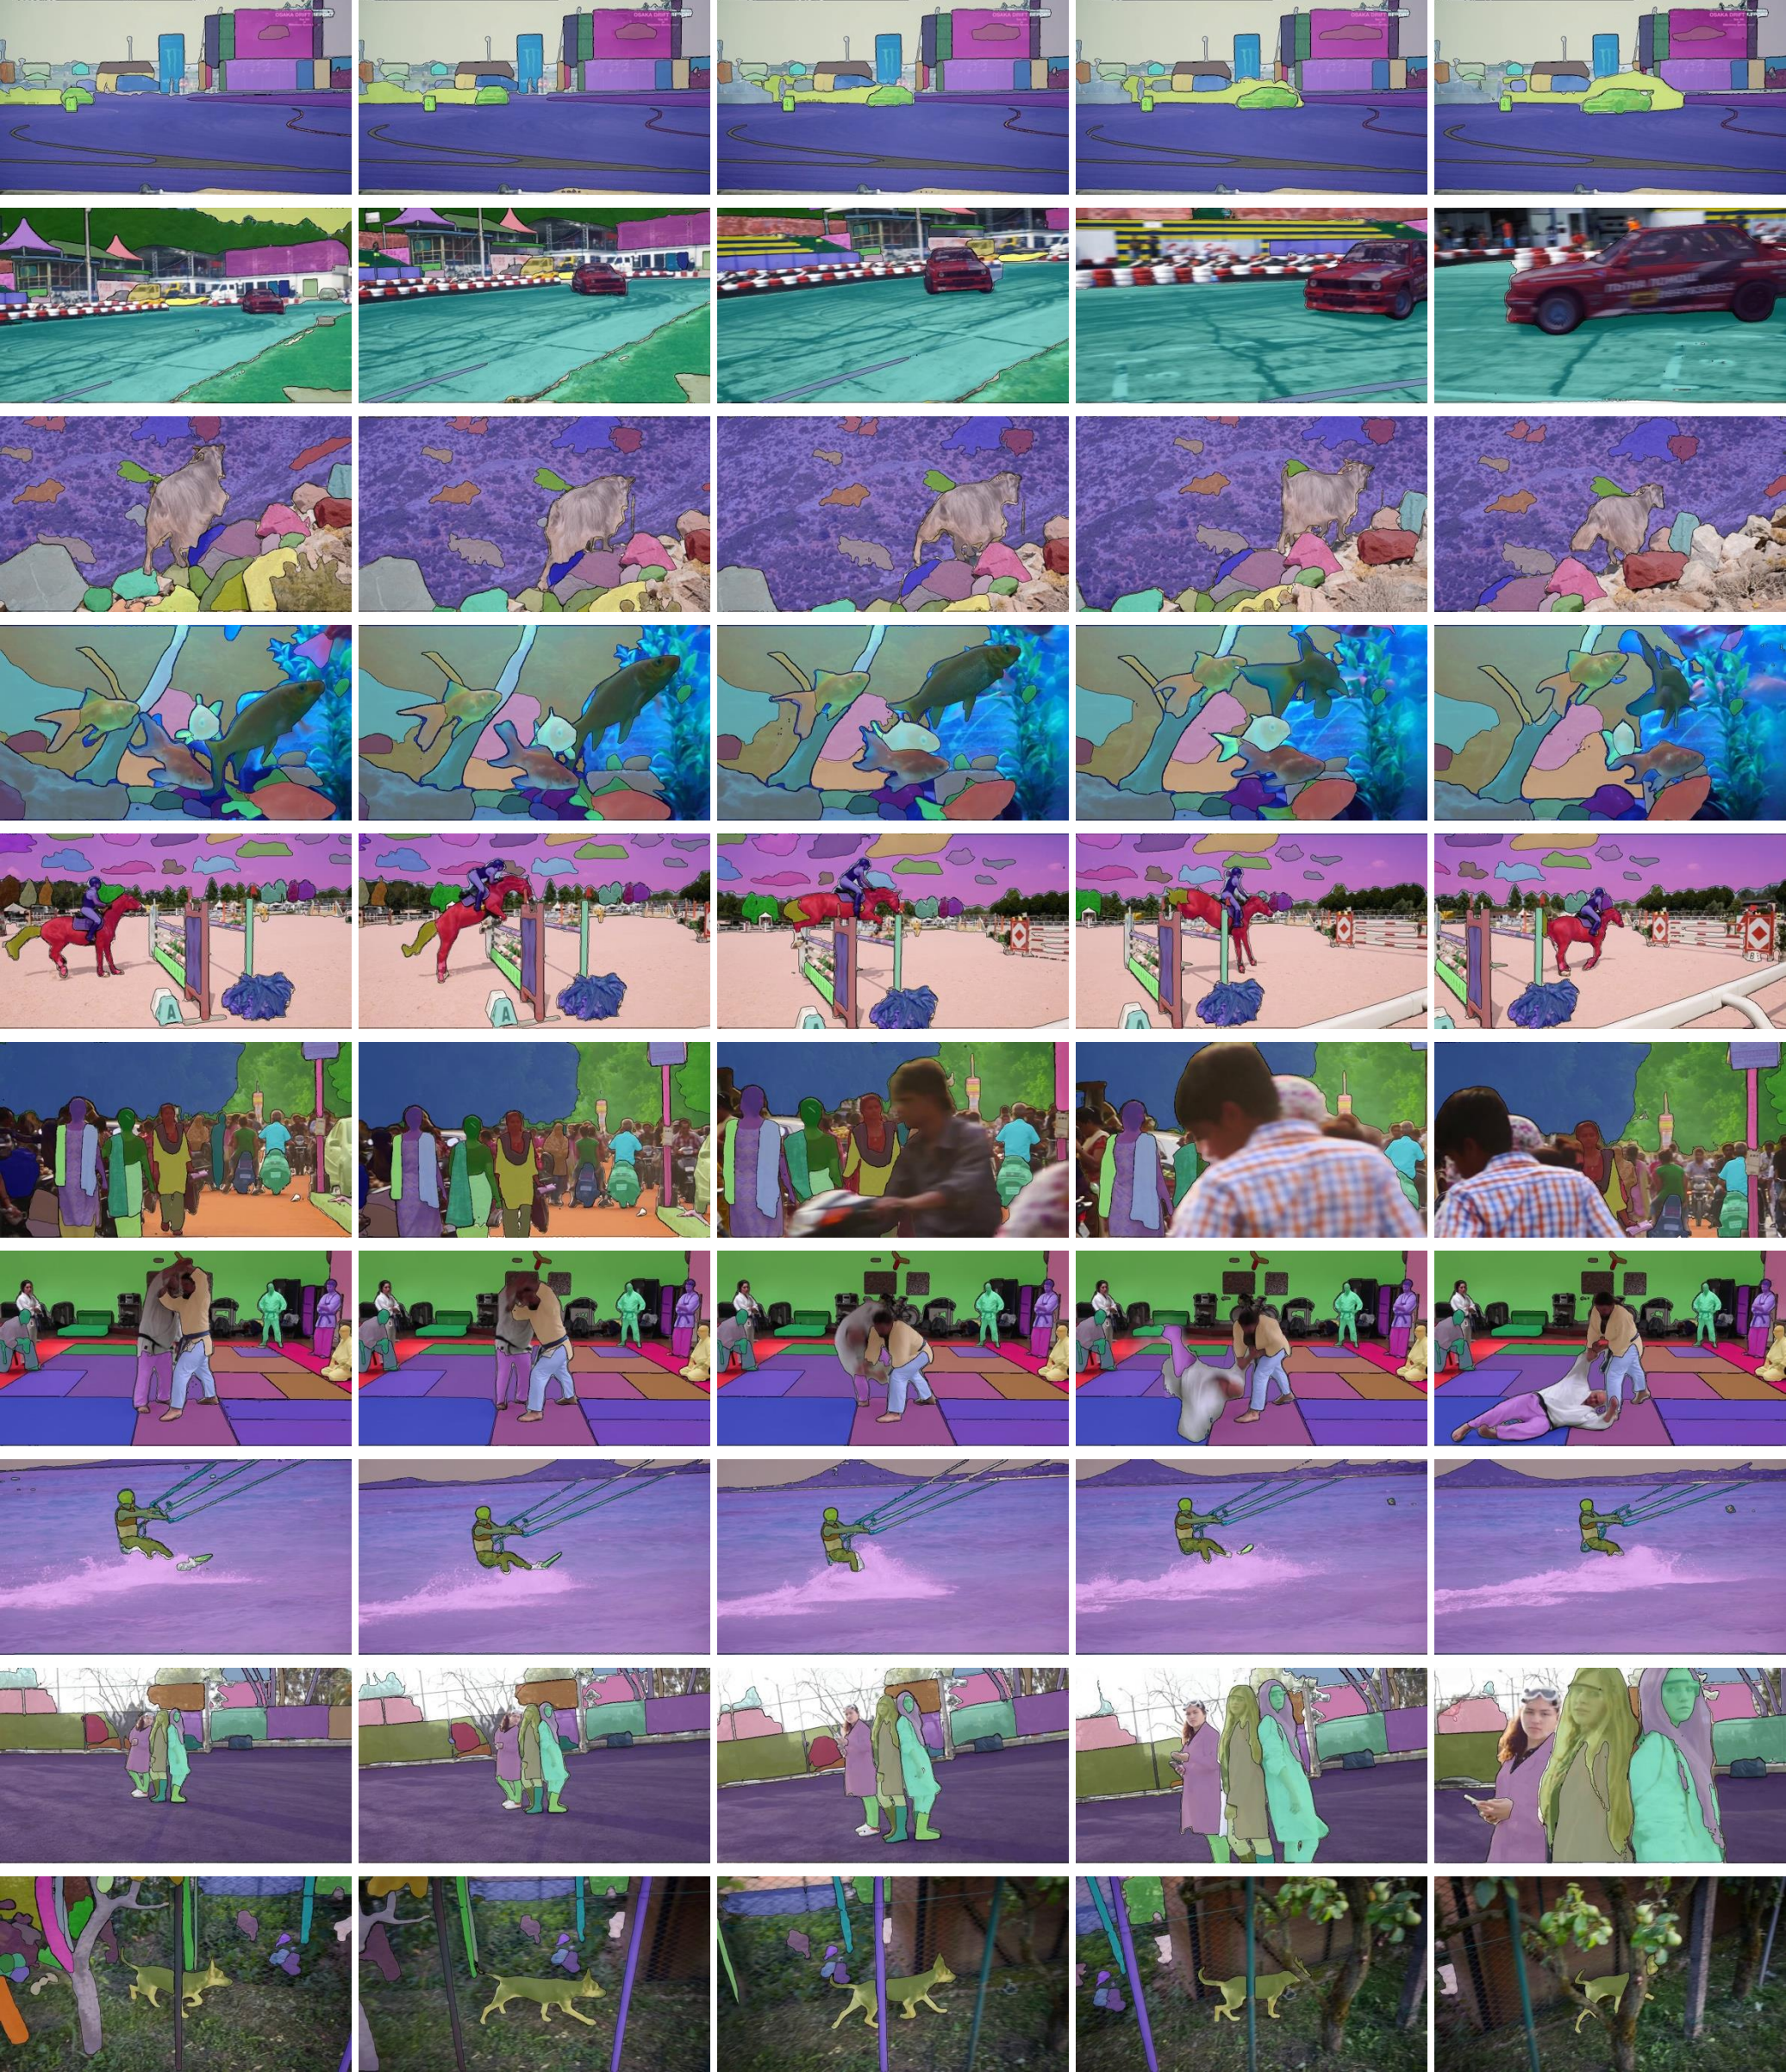



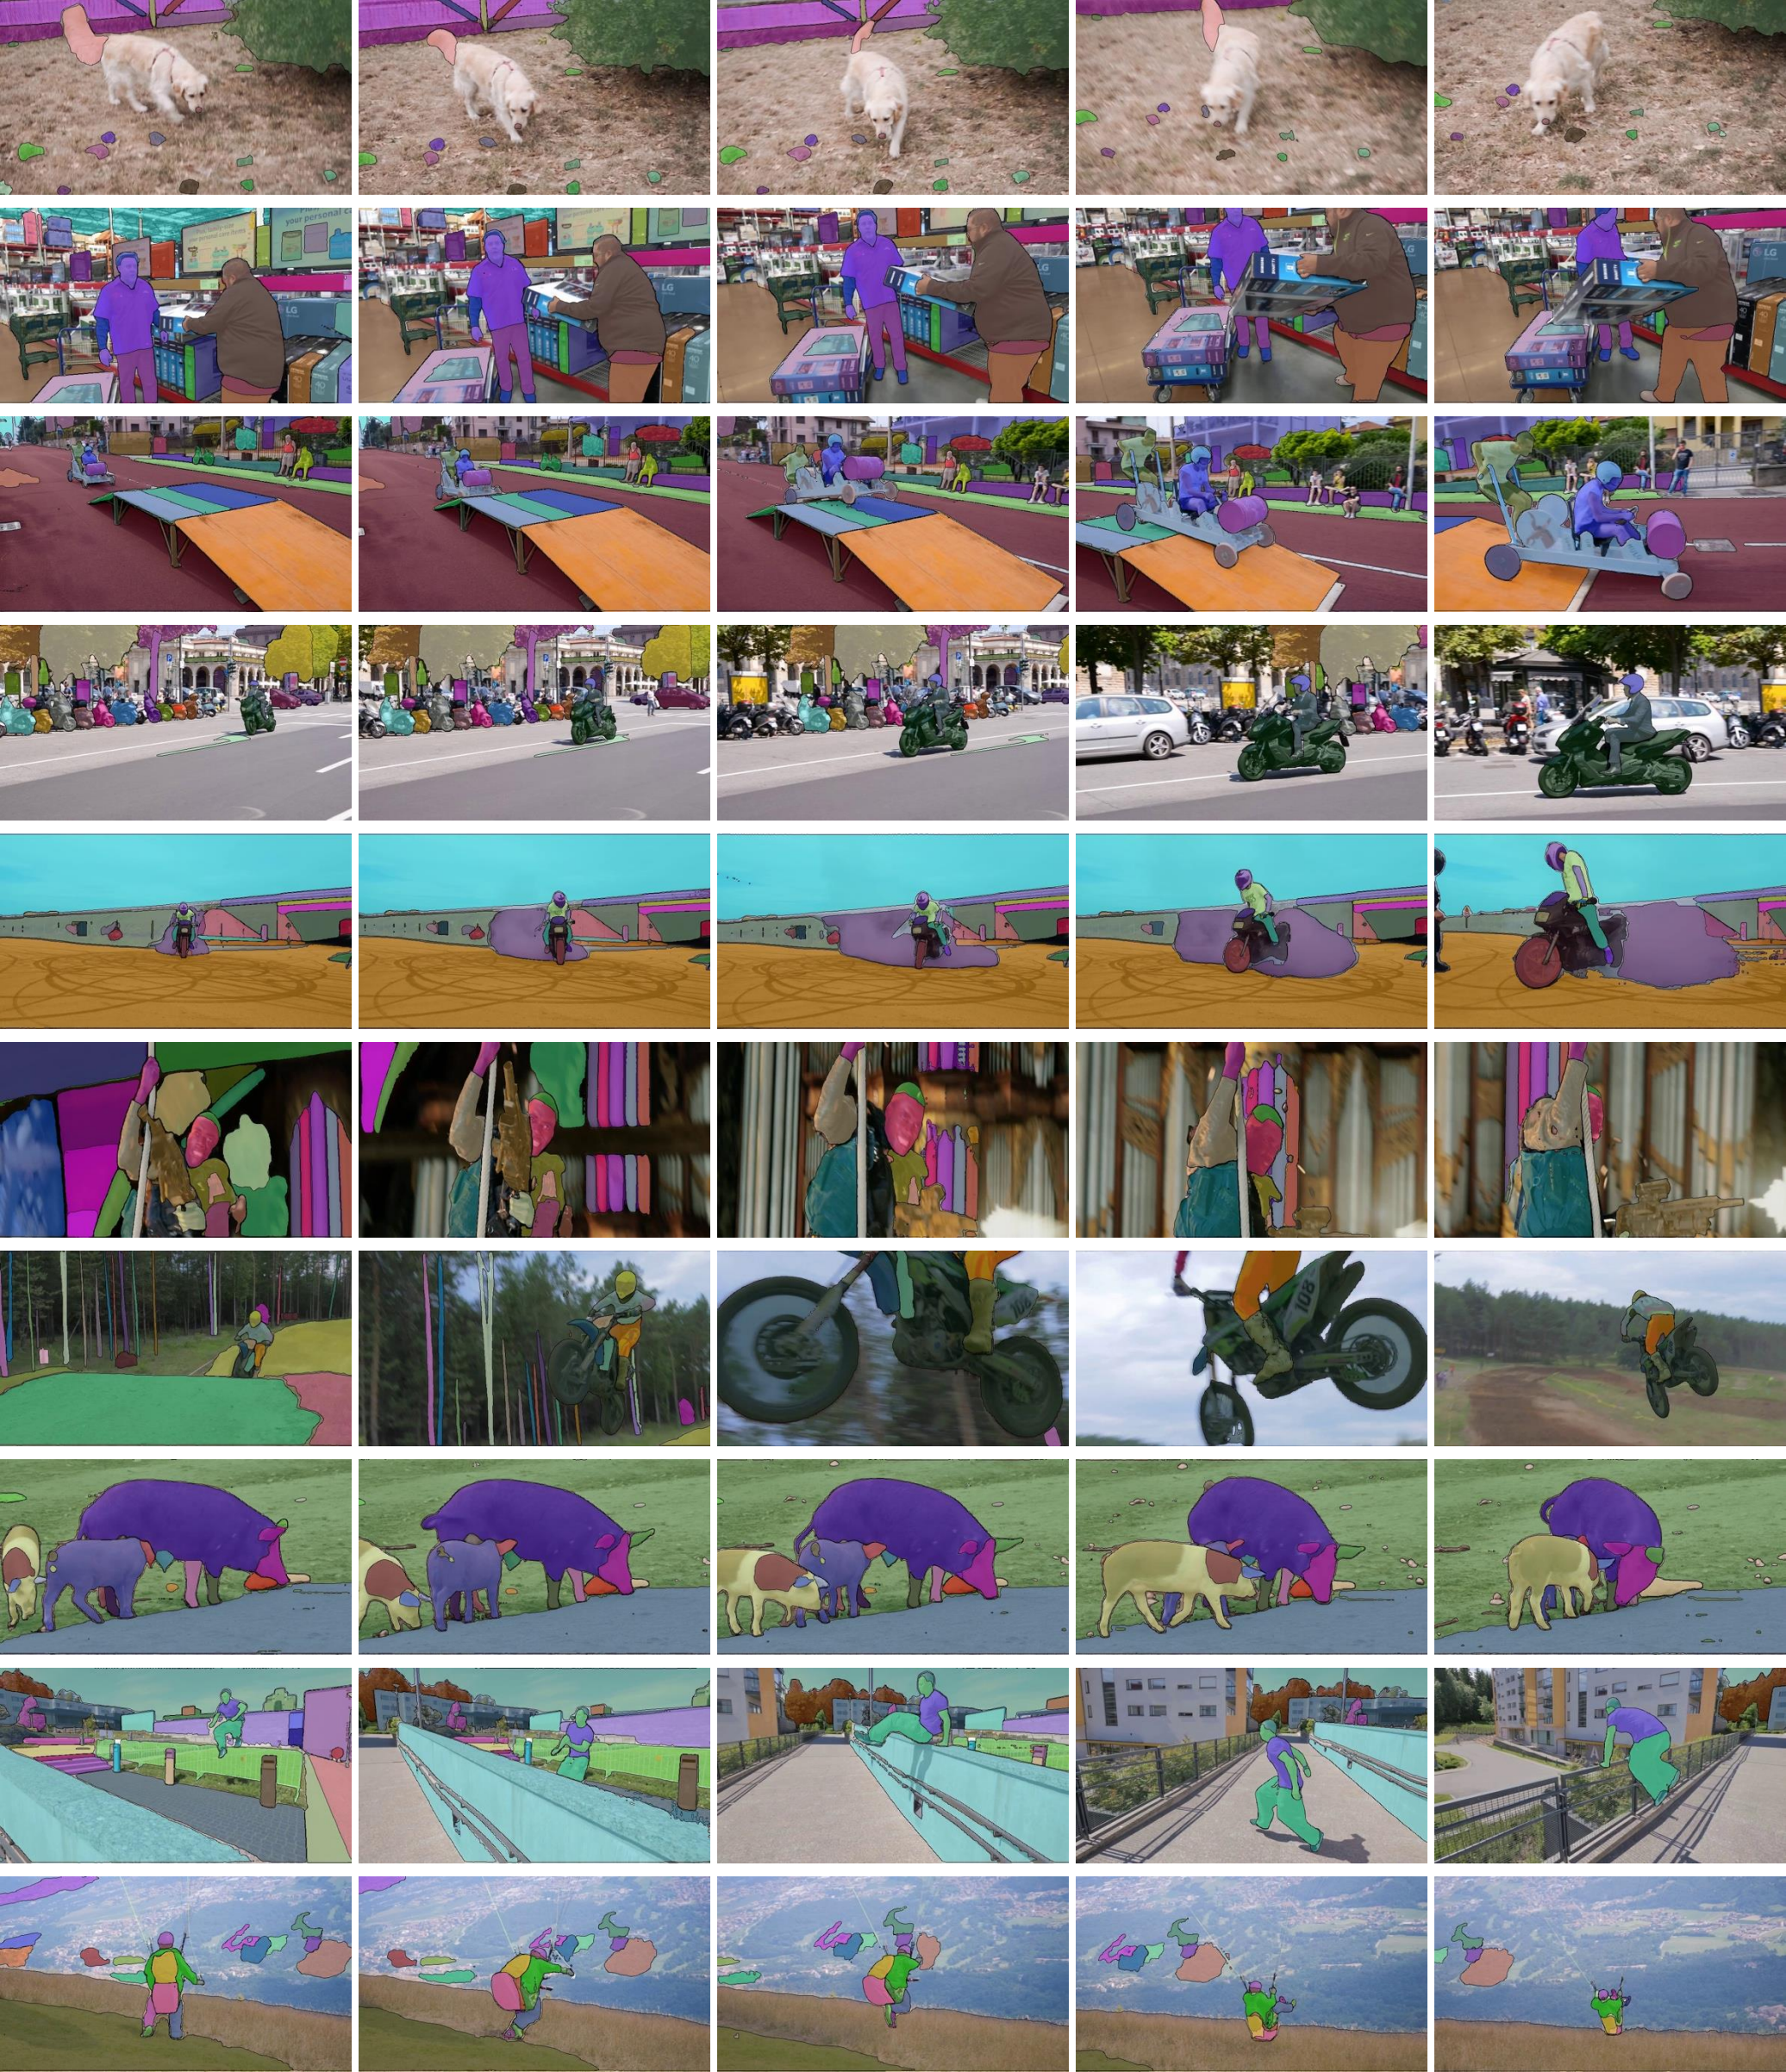

Supplement: Supplementary file 2 [file mug_test_0.pdf]
